# Supplementary material for: Towards Tackling MaxSAT by Combining Nested Monte Carlo with Local Search
Source: arXiv:2302.13225 source file (2023-02-26)
Supplement: Supplementary file 1 [file appendix.tex]

\section*{Appendix}
\subsection{Algorithms}

\subsection{Figures}

\begin{figure}[!tbh]
\centering
\hspace*{-1.5em}
\subfigure[random-no]{\label{subfig:orientation_mcts_walksat_random_no}
\resizebox{0.45\linewidth}{!}{\input{plots/rn_mcts_walksat.tex}}
}
\hspace*{-1.5em}
\subfigure[random-yes]{\label{subfig:orientation_mcts_walksat_random_yes}
\resizebox{0.45\linewidth}{!}{\input{plots/ry_mcts_walksat.tex}}
}

\hspace*{-1.5em}
\subfigure[global-no]{\label{subfig:orientation_mcts_walksat_global_no}
\resizebox{0.45\linewidth}{!}{\input{plots/gn_mcts_walksat.tex}}
}
\hspace*{-1.5em}
\subfigure[global-yes]{\label{subfig:orientation_mcts_walksat_global_yes}
\resizebox{0.45\linewidth}{!}{\input{plots/gy_mcts_walksat.tex}}
}
\caption{Walksat Based MCTS, the curve categorized by the fliplimits $fl$, the x-axis represents the time cost with the MCTS simulation. In this experiments, the MCTS simulation increases 25 from 50 to 150, which are marked in curves.}
\label{fig:orientation_mcts_walksat_gryn} 
\end{figure}  

For Walksat based MCTS in Fig~\ref{fig:orientation_mcts_walksat_gryn}, Comparing panel (a) with (b), and panel (c) with (d), we see using the best solution ever found by walksat as the final result of walksat contributes to the performance. Comparing panel (a) with (c), and panel (b) with (d), we see if the walksat is initialized based on the global best solution, then the performs improve. Clearly, using the best solution ever found by walksat is more important than initializing based on the global best solution according to panel (b) and (c). And the best combination is to implement both two components. 

Interestingly, for Walksat based NMC in Fig~\ref{fig:orientation_nest_walksat_gryn}, we see the same pattern, which is because the performance of both MCTS and NMC are highly depended on the quality of estimation of the state, and both components improves the estimation results. In particular, using the best solution ever found by walksat guarantee the upper bounds that walksat can find as the final result for estimation since the walksat might flip to a worse result during flipping step. In addition, for initializing walksat using the global best solution can speed up the flip process and avoid repeat flips. Therefore, in the following experiments, we adopt these two components.
 
\begin{figure}[!tbh]
\centering
\hspace*{-1.5em}
\subfigure[random-no]{\label{subfig:orientation_nest_walksat_random_no}
\resizebox{0.45\linewidth}{!}{\input{plots/rn_nest_walksat.tex}}
}
\hspace*{-1.5em}
\subfigure[random-yes]{\label{subfig:orientation_nest_walksat_random_yes}
\resizebox{0.45\linewidth}{!}{\input{plots/ry_nest_walksat.tex}}
}

\hspace*{-1.5em}
\subfigure[global-no]{\label{subfig:orientation_nest_walksat_global_no}
\resizebox{0.45\linewidth}{!}{\input{plots/gn_nest_walksat.tex}}
}
\hspace*{-1.5em}
\subfigure[global-yes]{\label{subfig:orientation_nest_walksat_global_yes}
\resizebox{0.45\linewidth}{!}{\input{plots/gy_nest_walksat.tex}}
}
\caption{Walksat Based NMC, the curve categorized by the fliplimits $fl$, the x-axis represents the time cost with the different repetitions. In this experiments, the NMC repetition increases 1 from 1 to 5, which are marked in curves.}
\label{fig:orientation_nest_walksat_gryn} 
\end{figure}  

From Fig.~\ref{fig:orientation_nest_dyn_walksat} and Fig.~\ref{subfig:orientation_nest_walksat_global_yes}, we see that in 1000 seconds, the dynamic $fl$ in Fig.~\ref{subfig:orientation_nest_dynwe_walksat} achieves the better performance. Fig.~\ref{subfig:orientation_mcts_dynwe_walksat} shows that given a fixed repetition for NMC, higher exponent gets better performance, and higher $w$ also gets better performance, this is because both higher exponent and higher $w$ lead to larger $fl$, larger $fl$ is more likely to get better estimation result. However, enlarging the exponent results in a quick consumption of time budget. In Fig.~\ref{subfig:orientation_mcts_dynws_walksat}, we see that setting exponent as 1, and increasing the MCTS simulation achieves the best performance within a small budget~(around 400 seconds). Therefore, in the full experiments, we set exponent as 1 for NMC and determine the repetition according to the budget.

\begin{figure}[!tbh]
\centering
\hspace*{-1.5em}
\subfigure[one repetition, exponent increases]{\label{subfig:orientation_nest_dynwe_walksat}
\resizebox{0.45\linewidth}{!}{\input{plots/nest_dynwe_walksat}}
}
\hspace*{-1.5em}
\subfigure[exponent=1, repetition increases]{\label{subfig:orientation_nest_dynwr_walksat}
\resizebox{0.45\linewidth}{!}{\input{plots/nest_dynwr_walksat}}
}
\caption{NMC with Dynamic Flip Limits for Walksat.
}
\label{fig:orientation_nest_dyn_walksat} 
\end{figure}

\subsection{Tables}
\begin{table*}[tbh!]
\hspace{-10cm}
\scriptsize
\caption{Results of Mastering Max3Sat~(70 variables) on different Instances Using SingleUCT SLS, MultiUCT SLS and NMC SLS respectively, 10 repetitions each. }\label{max3sat70variable_sls}
\resizebox{\textwidth}{!}{\input{tables/fullexperiments_70v}}
\end{table*}

%\begin{table}[tbh!]
%\hspace{-10cm}
%\scriptsize
%\caption{Results of Mastering Max3Sat~(80 variables) on different Instances Using SingleUCT SLS, MultiUCT SLS and NMC SLS respectively, 10 repetitions each. }\label{max3sat80variable_sls}
%\resizebox{\textwidth}{!}{\input{tables/fullexperiments_80v}}
%\end{table}

\begin{table*}[tbh!]
\hspace{-10cm}
\scriptsize
\caption{Results of Mastering Max2Sat~(120 variables) on different Instances Using SingleUCT SLS, MultiUCT SLS and NMC SLS respectively, 10 repetitions each. }\label{max2sat120variable_sls}
\resizebox{\textwidth}{!}{\input{tables/fullexperiments_120v}}
\end{table*}

\begin{table*}[tbh!]
\hspace{-10cm}
\scriptsize
\caption{Results of Mastering Max2Sat~(140 variables) on different Instances Using SingleUCT SLS, MultiUCT SLS and NMC SLS respectively, 10 repetitions each. }\label{max2sat140variable_sls}
\resizebox{\textwidth}{!}{\input{tables/fullexperiments_140v}}
\end{table*}

\begin{table*}[tbh!]
\hspace{-10cm}
\scriptsize
\caption{Results of Mastering Max2Sat~(200 variables) on different Instances Using SingleUCT SLS, MultiUCT SLS and NMC SLS respectively, 10 repetitions each. }\label{max2sat200variable_walksat}
\resizebox{\textwidth}{!}{\input{tables/fullexperiments_200v}}
\end{table*}

\begin{table*}[tbh!]
\hspace{-10cm}
\scriptsize
\caption{Results of Mastering Max2Sat~(250 variables) on different Instances Using SingleUCT SLS, MultiUCT SLS and NMC SLS respectively, 10 repetitions each. }\label{max2sat250variable_walksat}
\resizebox{\textwidth}{!}{\input{tables/fullexperiments_250v}}
\end{table*}

\begin{table*}[tbh!]
\hspace{-10cm}
\scriptsize
\caption{Results of Mastering Max2Sat~(300 variables) on different Instances Using SingleUCT SLS, MultiUCT SLS and NMC SLS respectively, 10 repetitions each. }\label{max2sat300variable_walksat}
\resizebox{\textwidth}{!}{\input{tables/fullexperiments_300v}}
\end{table*}

\subsection{Flip or Search Trade off}\label{subsect:flipvssearch}

Demonstrating that Nested makes better use of time than walksat

Does NMC-walksat benefit from doing more flips?

How to do dynamic setting of flips help NMC-walksat?

In dynamic setting, how best to use additional budget? More reps or more flips?

For MCTS-walksat, how best to use additional budget? More simulations or more flips?

\begin{figure*}[!tbh]
\centering
\hspace*{-1.5em}
\subfigure[]{\label{subfig:orientation_124}
\resizebox{0.45\linewidth}{!}{\input{plots/124}}
}
\hspace*{-1.5em}
\subfigure[]{\label{subfig:orientation_345}
\resizebox{0.45\linewidth}{!}{\input{plots/345}}
}
\hspace*{-1.5em}
\subfigure[]{\label{subfig:orientation_496}
\resizebox{0.45\linewidth}{!}{\input{plots/496}}
}
\hspace*{-1.5em}
\subfigure[]{\label{subfig:orientation_4678}
\resizebox{0.45\linewidth}{!}{\input{plots/4678}}
}
\hspace*{-1.5em}
\subfigure[]{\label{subfig:orientation_41011}
\resizebox{0.45\linewidth}{!}{\input{plots/41011}}
}

\caption{
}
\label{fig:orientation_tradeoff} 
\end{figure*}
